# Supplementary material for: C-PMI: Conditional Pointwise Mutual Information for Turn-level Dialogue Evaluation
Source: arXiv:2306.15245 source file (2023-09-01)
Supplement: Supplementary file 1 [file 700appendix.tex]

\clearpage
\section{Appendix}

\vicki{@Mankeerat: What's the point to include this table?}

\label{appendix:metrics}
\begin{table*}[!htb]
\small
    \centering
    \begin{tabular}{l|cccc}
    \toprule
    Metric & Pretrained Model & Training Dataset  & Reference-Free? & Objective \\
    \midrule
    BLEU \shortcite{papineni-etal-2002-bleu} & \xmark &  \xmark & \xmark & \xmark \\
    METEOR \shortcite{banerjee-lavie-2005-meteor} & \xmark &  \xmark & \xmark & \xmark \\
    ROUGE \shortcite{lin-2004-rouge} & \xmark &  \xmark & \xmark & \xmark \\
    ADEM \shortcite{lowe-etal-2017-towards} & \xmark & Ubuntu Dialogue + Twitter & \xmark & MSE \\
    BERTScore \shortcite{zhang2019bertscore} & BERT & \xmark & \xmark & \xmark \\
    BLEURT \shortcite{sellam-etal-2020-bleurt} & BERT & WMT Metrics Shared Task & \xmark & MSE \\
    QuestEval \shortcite{scialom2021questeval} & T5 &  SQuAD-v2/NewsQA & \checkmark  & QA/QG \\
    RUBER \shortcite{tao2018ruber} & \xmark & DailyDialog / PersonaChat & \xmark & Triplet  \\
    BERT-RUBER \shortcite{ghazarian-etal-2019-better} & BERT & DailyDialog / PersonaChat & \xmark & Triplet \\
    PONE \shortcite{10.1145/3423168} & BERT & DailyDialog & \xmark & Triplet \\
    MAUDE \shortcite{sinha-etal-2020-learning} & BERT & PersonaChat & \checkmark & NCE \\
        DEB  \shortcite{sai-etal-2020-improving} & BERT & Reddit/DailyDialog++ & \checkmark & MLM/NSP \\
        GRADE \shortcite{huang-etal-2020-grade} & BERT & DailyDialog & \checkmark & Triplet  \\
        DynaEval \shortcite{zhang-etal-2021-DynaEval} & RoBERTa & ED/ConvAI2/DailyDialog & \checkmark & Triplet \\
        USR \shortcite{mehri-eskenazi-2020-usr} & RoBERTa & TopicalChat / PersonaChat & \checkmark & MLM/CrossEntropy \\
        USL-H \shortcite{phy-etal-2020-deconstruct} & BERT & DailyDialog & \checkmark & VUP/NSP/MLM \\
        DialogRPT    \shortcite{gao2020dialogrpt} & GPT-2 & Reddit & \checkmark & CrossEntropy \\
        Deep AM-FM \shortcite{zhang2021deep} & Multilingual BERT & Twitter & \xmark & MLM \\ 
    HolisticEval \shortcite{pang-etal-2020-towards} & BERT & DailyDialog & \checkmark & LM \\
    PredictiveEngage \shortcite{ghazarian2020predictive} & BERT & ConvAI & \xmark & CrossEntropy \\
    FED \shortcite{mehri-eskenazi-2020-unsupervised} & DialoGPT & \xmark & \checkmark & \xmark  \\
    FlowScore \shortcite{li2021dialoflow} & Plato & Reddit & \checkmark & ContextFlow \\
    FBD \shortcite{xiang2021assessing} & RoBERTa & \xmark & \xmark & \xmark \\

    \bottomrule
     \end{tabular}
    \caption{This table provides a summary of the evaluation metrics used to assess the quality of dialog systems. The information presented here is primarily sourced from a comprehensive survey on dialog evaluation~\cite{yeh-etal-2021-comprehensive}. COPIED: The `Pretrained Model' column indicates the specific pretrained language model used by the metric. The `Training Dataset' and `Objective' columns describe the dialog data and the objective used when training the metric. `Reference-Free?' indicates whether the metric requires a reference response for evaluation. ED is the abbreviation of the EmpatheticDialogue dataset. }
    \label{tab:metric_overview}
\end{table*}
